# Supplementary material for: Economic Impacts of Climate Change in the United States: Integrating and Harmonizing Evidence from Recent Studies
Source: arXiv:2509.00212 source file (2026-10-08)
Supplement: Supplementary file 1 [file tab_ranking_gcms_all.tex]

INM-CM5-0 & 1.39 & 1.92 & 1.21 & 1 & 1 & 1 \\
\rowcolor{DarkSeaGreen1} NorESM2-LM & 1.48 & 2.6 & 1.43 & 2 & 4 & 2 \\
MIROC6 & 1.55 & 2.57 & 1.46 & 5 & 3 & 3 \\
CAMS-CSM1-0 & 1.75 & 2.29 & 1.48 & 9 & 2 & 4 \\
MIROC-ES2L & 1.55 & 2.68 & 1.49 & 4 & 6 & 5 \\
GFDL-ESM4 & 1.61 & 2.62 & 1.5 & 6 & 5 & 6 \\
BCC-CSM2-MR & 1.5 & 3.01 & 1.55 & 3 & 8 & 7 \\
MPI-ESM1-2-HR & 1.65 & 2.97 & 1.62 & 8 & 7 & 8 \\
MRI-ESM2-0 & 1.64 & 3.14 & 1.66 & 7 & 9 & 9 \\
GFDL-CM4 & 2.01 & 3.87 & 2.04 & 11 & 10 & 10 \\
CNRM-ESM2-1 & 1.9 & 4.7 & 2.2 & 10 & 14 & 11 \\
EC-Earth3 & 2.32 & 4.2 & 2.28 & 14 & 11 & 12 \\
CNRM-CM6-1 & 2.13 & 4.83 & 2.35 & 13 & 15 & 13 \\
CESM2 & 2.06 & 5.19 & 2.41 & 12 & 16 & 14 \\
EC-Earth3-Veg & 2.61 & 4.3 & 2.45 & 15 & 12 & 15 \\
NESM3 & 2.79 & 4.68 & 2.64 & 18 & 13 & 16 \\
UKESM1-0-LL & 2.75 & 5.34 & 2.8 & 17 & 17 & 17 \\
CanESM5 & 2.66 & 5.62 & 2.83 & 16 & 18 & 18 \\
\bottomrule
